# Supplementary material for: Evaluation of Neel temperatures from fully self-consistent broken-symmetry GW and high-temperature expansion: application to cubic transition-metal oxides
Source: arXiv:2209.14904 source file (2023-03-20)
Supplement: Supplementary file 1 [file SI.pdf]

# Evaluation of Neel temperatures from fully self-consistent broken-symmetry GW and high-temperature expansion: application to cubic transition-metal oxides

Pavel Pokhilko[1] and Dominika Zgid[1,2]

[1]*Department of Chemistry, University of Michigan, Ann Arbor, Michigan 48109, USA*

[2]*Department of Physics, University of Michigan, Ann Arbor, Michigan 48109, USA*

## 1. VALIDATION

To validate the approach, we considered two limiting cases for $s = 1/2$.

**Case 1**. If $J_1 = 0$, only NNN centers are coupled with $J_2$ constant. Because of the nature of this coupling, the lattice is represented by simple cubic sublattices, which do not interact with each other. To validate the approach, we can compare only with the simple cubic lattices. Because of the structure of polynomials with only one coupling constant, the ferro- and antiferromagnetic cases are exactly equivalent (we do not consider staggered susceptibility in this work).

Rushbrooke and Wood[1] used the following form of Hamiltonian $H = -\frac{1}{2} J_{RW} \sum_{\langle i,j \rangle} \sigma_i \sigma_j$ and got an extrapolated estimate for a cubic lattice: $T_C^{RW} = 1.92 J_{RW}$. Domb and Sykes[2] got an estimate: $T_C^{DS} = 1.83 J_{RW}$.

Since $S = \sigma/2$, the relation with our form is $J_{RW} = J/2$ and $T_C^{RW} = 0.96J$, $T_C^{DS} = 0.915J$. Table S1 shows convergence of our estimates. From our calculations, the ratios $q_4$ and $q_5$ give very close estimates to Domb and Sykes; however, the higher-order terms reduce the estimate.

Ref.[3] provides a QMC estimate $T_C^{TAW} = 0.947J$, which is consistent with the ones from Refs.[1, 2].

**Case 2.** If $J_2 = 0$, only NN centers are coupled with $J_1$ constant. This case is an fcc lattice. The Rushbrooke and Wood estimate[1] for this lattice is $T_C^{RW} = 4.21 J_{RW}$; the Domb and Sykes estimate[2] is $T_C^{DS} = 4.17 J_{RW}$. In our notation, $T_C^{RW} = 2.105J$ and $T_C^{DS} = 2.085J$. The $h_n$ overshoots the previous estimates quite a bit, but the ratio test seems to be working well.

TABLE S1: Multiplicator $m$ for $T_N = m \cdot J_2$ for spin 1/2 and $J_1 = 0$ from $\chi$.

| $n$ | $q_n$ | $\frac{nq_n}{n-1}$ | $g_n$ | $h_n$ |
|---|---|---|---|---|
| 2 | 1.5000 | 3.0000 | 0.3750 | 0.7500 |
| 3 | 1.0000 | 1.5000 | 0.6124 | 1.0607 |
| 4 | 0.9167 | 1.2222 | 0.7005 | 1.1120 |
| 5 | 0.9375 | 1.1719 | 0.7534 | 1.1267 |
| 6 | 0.9461 | 1.1353 | 0.7885 | 1.1284 |
| 7 | 0.8812 | 1.0281 | 0.8033 | 1.1110 |
| 8 | 0.8682 | 0.9923 | 0.8123 | 1.0932 |
| 9 | 0.9050 | 1.0181 | 0.8233 | 1.0835 |
| 10 | 0.8956 | 0.9951 | 0.8310 | 1.0733 |

TABLE S2: Multiplicator $m$ for $T_N = m \cdot J_1$ for spin 1/2 and $J_2 = 0$ from $\chi$.

| $n$ | $q_n$ | $\frac{nq_n}{n-1}$ | $g_n$ | $h_n$ |
|---|---|---|---|---|
| 2 | 3.0000 | 6.0000 | 0.7500 | 1.5000 |
| 3 | 2.5000 | 3.7500 | 1.3693 | 2.3717 |
| 4 | 2.3000 | 3.0667 | 1.6277 | 2.5838 |
| 5 | 2.2147 | 2.7683 | 1.7580 | 2.6288 |
| 6 | 2.1747 | 2.6096 | 1.8344 | 2.6249 |
| 7 | 2.1501 | 2.5085 | 1.8836 | 2.6052 |
| 8 | 2.1311 | 2.4355 | 1.9171 | 2.5802 |
| 9 | 2.1153 | 2.3797 | 1.9408 | 2.5543 |
| 10 | 2.1027 | 2.3363 | 1.9582 | 2.5291 |

## 2. HIGH-TEMPERATURE EXPANSION

### 2.1. $S = 1/2$

Susceptibility:

$$c_1/N = +1/4$$

$$c_2/N = -3/4J_1 - 3/8J_2$$

$$c_3/N = +15/8J_1^2 + 9/4J_1J_2 + 3/8J_2^2$$

$$c_4/N = -69/16J_1^3 - 273/32J_1^2J_2 - 63/16J_1J_2^2 - 11/32J_2^3$$

$$c_5/N = +2445/256J_1^4 + 1683/64J_1^3J_2 + 2793/128J_1^2J_2^2 + 87/16J_1J_2^3 + 165/512J_2^4$$

$$\begin{aligned} c_6/N = &-53171/2560J_1^5 - 2333/32J_1^4J_2 - 22725/256J_1^3J_2^2 \\ &- 10637/256J_1^2J_2^3 - 1719/256J_1J_2^4 - 1561/5120J_2^5 \end{aligned}$$

$$\begin{aligned} c_7/N = &+914601/20480J_1^6 + 487343/2560J_1^5J_2 + 3118101/10240J_1^4J_2^2 \\ &+ 111543/512J_1^3J_2^3 + 679573/10240J_1^2J_2^4 + 5007/640J_1J_2^5 + 33013/122880J_2^6 \end{aligned}$$

$$\begin{aligned} c_8/N = &-4093045/43008J_1^7 - 9783881/20480J_1^6J_2 - 29003603/30720J_1^5J_2^2 - 112366097/122880J_1^4J_2^3 \\ &- 13367599/30720J_1^3J_2^4 - 1166447/12288J_1^2J_2^5 - 177649/20480J_1J_2^6 - 100321/430080J_2^7 \end{aligned}$$

$$\begin{aligned} c_9/N = &+461758903/2293760J_1^8 + 500503211/430080J_1^7J_2 + 3141838327/1146880J_1^6J_2^2 \\ &+ 2874263461/860160J_1^5J_2^3 + 252789671/114688J_1^4J_2^4 + 648894413/860160J_1^3J_2^5 \\ &+ 433476061/3440640J_1^2J_2^6 + 2643601/286720J_1J_2^7 + 968407/4587520J_2^8 \end{aligned}$$

$$\begin{aligned} c_{10}/N = &-546144169/1290240J_1^9 - 3176599023/1146880J_1^8J_2 - 8685678683/1146880J_1^7J_2^2 \\ &- 229917930491/20643840J_1^6J_2^3 - 64848524381/6881280J_1^5J_2^4 - 4457889623/983040J_1^4J_2^5 \\ &- 8137676399/6881280J_1^3J_2^6 - 1087155049/6881280J_1^2J_2^7 - 1563921/163840J_1J_2^8 \\ &- 23417483/123863040J_2^9 \end{aligned}$$

Heat capacity:

$$
\begin{aligned}
d_1/N =& 0\\
d_2/N =& + 9/8 J_1^2 + 9/16 J_2^2\\
d_3/N =& - 27/16 J_1^3 - 27/8 J_1^2 J_2 + 9/32 J_2^3\\
d_4/N =& + 45/128 J_1^4 + 9 J_1^3 J_2 + 9/8 J_1^2 J_2^2 - 81/256 J_2^4\\
d_5/N =& + 105/128 J_1^5 - 195/32 J_1^4 J_2 - 585/32 J_1^3 J_2^2 - 15/16 J_1^2 J_2^3 - 105/256 J_2^5\\
d_6/N =& + 3375/2048 J_1^6 - 621/128 J_1^5 J_2 + 43713/1024 J_1^4 J_2^2 + 3105/128 J_1^3 J_2^3 + 7047/1024 J_1^2 J_2^4\\
& + 1383/4096 J_2^6\\
d_7/N =& - 30345/4096 J_1^7 - 10563/1280 J_1^6 J_2 - 157857/5120 J_1^5 J_2^2 - 605073/5120 J_1^4 J_2^3\\
& - 354501/10240 J_1^3 J_2^4 - 72639/10240 J_1^2 J_2^5 + 21231/40960 J_2^7\\
d_8/N =& + 1955741/163840 J_1^8 + 376989/5120 J_1^7 J_2 + 717973/20480 J_1^6 J_2^2 + 1169781/5120 J_1^5 J_2^3\\
& + 2007513/10240 J_1^4 J_2^4 + 270163/5120 J_1^3 J_2^5 + 103/1024 J_1^2 J_2^6 - 54201/327680 J_2^8\\
d_9/N =& - 7614861/573440 J_1^9 - 201213/1280 J_1^8 J_2 - 12048849/40960 J_1^7 J_2^2\\
& - 80059611/286720 J_1^6 J_2^3 - 95676363/143360 J_1^5 J_2^4 - 41528799/143360 J_1^4 J_2^5\\
& - 290727/4480 J_1^3 J_2^6 - 195777/71680 J_1^2 J_2^7 - 89777/163840 J_2^9\\
d_{10}/N =& + 46528541/2621440 J_1^{10} + 46260349/229376 J_1^9 J_2 + 62172081/65536 J_1^8 J_2^2\\
& + 6394461/7168 J_1^7 J_2^3 + 2551803995/1835008 J_1^6 J_2^4 + 21970467/16384 J_1^5 J_2^5\\
& + 862640161/1835008 J_1^4 J_2^6 + 15893673/229376 J_1^3 J_2^7 + 20255043/1835008 J_1^2 J_2^8\\
& + 2253927/36700160 J_2^{10}
\end{aligned}
$$

## 2.2. $S = 1$

Susceptibility:

$$
\begin{aligned}
c_1/N &= +2/3 \\
c_2/N &= -16/3J_1 - 8/3J_2 \\
c_3/N &= +340/9J_1^2 + 128/3J_1J_2 + 74/9J_2^2 \\
c_4/N &= -6848/27J_1^3 - 4096/9J_1^2J_2 - 1952/9J_1J_2^2 - 656/27J_2^3 \\
c_5/N &= +133975/81J_1^4 + 110224/27J_1^3J_2 + 87832/27J_1^2J_2^2 + 24704/27J_1J_2^3 + 11215/162J_2^4 \\
c_6/N &= -12872224/1215J_1^5 - 8101232/243J_1^4J_2 - 9144560/243J_1^3J_2^2 - 4397456/243J_1^2J_2^3 \\
&\quad - 281384/81J_1J_2^4 - 237692/1215J_2^5 \\
c_7/N &= +488793583/7290J_1^6 + 935703316/3645J_1^5J_2 + 1370758798/3645J_1^4J_2^2 + 63451792/243J_1^3J_2^3 \\
&\quad + 315844694/3645J_1^2J_2^4 + 15011552/1215J_1J_2^5 + 878407/1620J_2^6 \\
c_8/N &= -2146891555/5103J_1^7 - 20758564832/10935J_1^6J_2 - 37438483904/10935J_1^5J_2^2 \\
&\quad - 11404609498/3645J_1^4J_2^3 - 16589892712/10935J_1^3J_2^4 - 821283908/2187J_1^2J_2^5 \\
&\quad - 50958092/1215J_1J_2^6 - 228464303/153090J_2^7 \\
c_9/N &= +3211964139551/1224720J_1^8 + 49681728994/3645J_1^7J_2 + 2236547137268/76545J_1^6J_2^2 \\
&\quad + 7625594149966/229635J_1^5J_2^3 + 983437262447/45927J_1^4J_2^4 + 597016105846/76545J_1^3J_2^5 \\
&\quad + 348028473839/229635J_1^2J_2^6 + 10528960936/76545J_1J_2^7 + 29935281917/7348320J_2^8 \\
c_{10}/N &= -14939510580089/918540J_1^9 - 65918415723383/688905J_1^8J_2 \\
&\quad - 655220039084497/2755620J_1^7J_2^2 - 99088994581687/306180J_1^6J_2^3 \\
&\quad - 240357370352203/918540J_1^5J_2^4 - 351844144494329/2755620J_1^4J_2^5 \\
&\quad - 50512095609593/1377810J_1^3J_2^6 - 2662639684501/459270J_1^2J_2^7 \\
&\quad - 28820879489/65610J_1J_2^8 - 61060471243/5511240J_2^9
\end{aligned}
$$

Heat capacity:

$$d_1/N = 0$$

$$d_2/N = +8J_1^2 + 4J_2^2$$

$$d_3/N = -116/3J_1^3 - 64J_1^2J_2 + 2J_2^3$$

$$d_4/N = +440/3J_1^4 + 1472/3J_1^3J_2 + 544/3J_1^2J_2^2 + 4J_2^4$$

$$d_5/N = -16670/27J_1^5 - 22240/9J_1^4J_2 - 9040/3J_1^3J_2^2 - 6560/9J_1^2J_2^3 - 55/27J_2^5$$

$$d_6/N = +232210/81J_1^6 + 343376/27J_1^5J_2 + 645724/27J_1^4J_2^2 + 131680/9J_1^3J_2^3 + 8804/3J_1^2J_2^4 + 5413/81J_2^6$$

$$\begin{aligned} d_7/N = &-2296469/162J_1^7 - 29338148/405J_1^6J_2 - 63256718/405J_1^5J_2^2 \\ &- 65691122/405J_1^4J_2^3 - 26082182/405J_1^3J_2^4 - 1463896/135J_1^2J_2^5 + 20209/540J_2^7 \end{aligned}$$

$$\begin{aligned} d_8/N = &+89464141/1215J_1^8 + 1552314784/3645J_1^7J_2 + 3740001232/3645J_1^6J_2^2 \\ &+ 183590608/135J_1^5J_2^3 + 3280352584/3645J_1^4J_2^4 + 967794368/3645J_1^3J_2^5 \\ &+ 8237768/243J_1^2J_2^6 + 1094167/7290J_2^8 \end{aligned}$$

$$\begin{aligned} d_9/N = &-39910675309/102060J_1^9 - 21351548768/8505J_1^8J_2 - 2778443377/405J_1^7J_2^2 \\ &- 267472705487/25515J_1^6J_2^3 - 79936455269/8505J_1^5J_2^4 - 37603640362/8505J_1^4J_2^5 \\ &- 8740244732/8505J_1^3J_2^6 - 130887716/1215J_1^2J_2^7 + 3783533/68040J_2^9 \end{aligned}$$

$$\begin{aligned} d_{10}/N = &+70909217363/34020J_1^{10} + 75496322222/5103J_1^9J_2 + 929637769547/20412J_1^8J_2^2 \\ &+ 134701829897/1701J_1^7J_2^3 + 124560164755/1458J_1^6J_2^4 + 283546546904/5103J_1^5J_2^5 \\ &+ 5053437379/252J_1^4J_2^6 + 6442510723/1701J_1^3J_2^7 + 6854041127/20412J_1^2J_2^8 + 49872199/34020J_2^{10} \end{aligned}$$

## 2.3. $S = 3/2$

Susceptibility:

$$c_1/N = +\,5/4$$

$$c_2/N = -\,75/4J_1 - 75/8J_2$$

$$c_3/N = +\,2025/8J_1^2 + 1125/4J_1J_2 + 225/4J_2^2$$

$$c_4/N = -\,52195/16J_1^3 - 182625/32J_1^2J_2 - 43875/16J_1J_2^2 - 10445/32J_2^3$$

$$c_5/N = +\,10486625/256J_1^4 + 6283275/64J_1^3J_2 + 9924825/128J_1^2J_2^2 + 359175/16J_1J_2^3 + 934025/512J_2^4$$

$$\begin{aligned} c_6/N = &-\,259040791/512J_1^5 - 49377505/32J_1^4J_2 - 437993805/256J_1^3J_2^2 - 212195725/256J_1^2J_2^3 \\ &-\,42531375/256J_1J_2^4 - 10343781/1024J_2^5 \end{aligned}$$

$$\begin{aligned} c_7/N = &+\,75922573739/12288J_1^6 + 11726657935/512J_1^5J_2 + 67179847085/2048J_1^4J_2^2 \\ &+\,11597471215/512J_1^3J_2^3 + 15723531445/2048J_1^2J_2^4 + 147731085/128J_1J_2^5 \\ &+\,1350478069/24576J_2^6 \end{aligned}$$

$$\begin{aligned} c_8/N = &-\,1609314345971/21504J_1^7 - 4015300465303/12288J_1^6J_2 - 3530120685743/6144J_1^5J_2^2 \\ &-\,12736162793789/24576J_1^4J_2^3 - 517797771467/2048J_1^3J_2^4 - 264690484925/4096J_1^2J_2^5 \\ &-\,31385968445/4096J_1J_2^6 - 2129486643/7168J_2^7 \end{aligned}$$

$$\begin{aligned} c_9/N = &+\,1239764440166389/1376256J_1^8 + 18549555999909/4096J_1^7J_2 \\ &+\,6501457098750917/688128J_1^6J_2^2 + 1814639396623673/172032J_1^5J_2^3 \\ &+\,2331763174511747/344064J_1^4J_2^4 + 431675603988721/172032J_1^3J_2^5 \\ &+\,349440190296845/688128J_1^2J_2^6 + 2821562478645/57344J_1J_2^7 \\ &+\,4383281372213/2752512J_2^8 \end{aligned}$$

$$\begin{aligned} c_{10}/N = &-\,33411396554597867/3096576J_1^9 - 42243061337032397/688128J_1^8J_2 \\ &-\,102034465653931511/688128J_1^7J_2^2 - 816001680672104435/4128768J_1^6J_2^3 \\ &-\,72576180891125731/458752J_1^5J_2^4 - 35601003109299027/458752J_1^4J_2^5 \\ &-\,31446299770617959/1376256J_1^3J_2^6 - 5214639932432965/1376256J_1^2J_2^7 \\ &-\,10088230347665/32768J_1J_2^8 - 210674954104387/24772608J_2^9 \end{aligned}$$

Heat capacity:

$$
\begin{aligned}
d_1/N =& 0 \\
d_2/N =& + 225/8J_1^2 + 225/16J_2^2 \\
d_3/N =& - 4275/16J_1^3 - 3375/8J_1^2J_2 + 225/32J_2^3 \\
d_4/N =& + 291645/128J_1^4 + 12375/2J_1^3J_2 + 21375/8J_1^2J_2^2 + 32895/256J_2^4 \\
d_5/N =& - 2611575/128J_1^5 - 2182875/32J_1^4J_2 - 2368125/32J_1^3J_2^2 - 344625/16J_1^2J_2^3 + 11175/256J_2^5 \\
d_6/N =& + 383973855/2048J_1^6 + 97009875/128J_1^5J_2 + 1214190225/1024J_1^4J_2^2 + 91864125/128J_1^3J_2^3 \\
& + 159645375/1024J_1^2J_2^4 + 14114055/4096J_2^6 \\
d_7/N =& - 7307256537/4096J_1^7 - 2193231285/256J_1^6J_2 - 16803355485/1024J_1^5J_2^2 \\
& - 15544990335/1024J_1^4J_2^3 - 12721010505/2048J_1^3J_2^4 - 2299867815/2048J_1^2J_2^5 \\
& + 15560643/8192J_2^7 \\
d_8/N =& + 576989776217/32768J_1^8 + 99198516201/1024J_1^7J_2 + 897188936433/4096J_1^6J_2^2 \\
& + 266248920985/1024J_1^5J_2^3 + 334407638961/2048J_1^4J_2^4 + 51266684355/1024J_1^3J_2^5 \\
& + 7274261925/1024J_1^2J_2^6 + 3414912443/65536J_2^8 \\
d_9/N =& - 20413490141033/114688J_1^9 - 7863418565109/7168J_1^8J_2 - 23446408084893/8192J_1^7J_2^2 \\
& - 233798471534487/57344J_1^6J_2^3 - 96683090030595/28672J_1^5J_2^4 - 44846931896055/28672J_1^4J_2^5 \\
& - 85057848675/224J_1^3J_2^6 - 92312736435/2048J_1^2J_2^7 + 7865195957/229376J_2^9 \\
d_{10}/N =& + 6691816120691119/3670016J_1^{10} + 2856247648288145/229376J_1^9J_2 \\
& + 16861556210344505/458752J_1^8J_2^2 + 3492957943879875/57344J_1^7J_2^3 \\
& + 16126937780118445/262144J_1^6J_2^4 + 4365534887299725/114688J_1^5J_2^5 \\
& + 25379119392941745/1835008J_1^4J_2^6 + 631057531018125/229376J_1^3J_2^7 \\
& + 500904514600475/1835008J_1^2J_2^8 + 8718660187179/7340032J_2^{10}
\end{aligned}
$$

### 2.4. $S = 2$

Susceptibility:

$$
\begin{aligned}
c_1/N =& + 2 \\
c_2/N =& - 48J_1 - 24J_2 \\
c_3/N =& + 1044J_1^2 + 1152J_1J_2 + 234J_2^2 \\
c_4/N =& - 108704/5J_1^3 - 37632J_1^2J_2 - 18144J_1J_2^2 - 11072/5J_2^3 \\
c_5/N =& + 2208667/5J_1^4 + 5228112/5J_1^3J_2 + 4114488/5J_1^2J_2^2 + 1205376/5J_1J_2^3 + 40391/2J_2^4 \\
c_6/N =& - 220857632/25J_1^5 - 664621232/25J_1^4J_2 - 731585424/25J_1^3J_2^2 - 71111696/5J_1^2J_2^3 \\
& - 14509752/5J_1J_2^4 - 4562124/25J_2^5 \\
c_7/N =& + 5242868069/30J_1^6 + 15970734284/25J_1^5J_2 + 22659542122/25J_1^4J_2^2 + 15615025712/25J_1^3J_2^3 \\
& + 5339225378/25J_1^2J_2^4 + 820698912/25J_1J_2^5 + 97256917/60J_2^6 \\
c_8/N =& - 1800643378049/525J_1^7 - 5535711712016/375J_1^6J_2 - 9629826487112/375J_1^5J_2^2 \\
& - 8640230032694/375J_1^4J_2^3 - 1408926703576/125J_1^3J_2^4 - 72989372132/25J_1^2J_2^5 \\
& - 8879440172/25J_1J_2^6 - 25047031309/1750J_2^7 \\
c_9/N =& + 561987572348731/8400J_1^8 + 290026824117186/875J_1^7J_2 + 1794236346768422/2625J_1^6J_2^2 \\
& + 1988538770366342/2625J_1^5J_2^3 + 1275984452698474/2625J_1^4J_2^4 + 95145217742282/525J_1^3J_2^5 \\
& + 97931101599179/2625J_1^2J_2^6 + 3253957166856/875J_1J_2^7 + 10525952900311/84000J_2^8 \\
c_{10}/N =& - 245469079935094 07/18900J_1^9 - 95560563627804973/13125J_1^8J_2 \\
& - 182403747566031569/10500J_1^7J_2^2 - 723000678902732437/31500J_1^6J_2^3 \\
& - 320242886814148447/17500J_1^5J_2^4 - 22495709695413429/2500J_1^4J_2^5 \\
& - 14057088295997141/5250J_1^3J_2^6 - 2378447765149453/5250J_1^2J_2^7 \\
& - 9488675110279/250J_1J_2^8 - 1032938179492699/945000J_2^9
\end{aligned}
$$

Heat capacity:

$$
\begin{aligned}
d_1/N =&0\\
d_2/N =&+72J_1^2+36J_2^2\\
d_3/N =&-1116J_1^3-1728J_1^2J_2+18J_2^3\\
d_4/N =&+81288/5J_1^4+40896J_1^3J_2+18720J_1^2J_2^2+5364/5J_2^4\\
d_5/N =&-243306J_1^5-764832J_1^4J_2-795600J_1^3J_2^2-247776J_1^2J_2^3+483J_2^5\\
d_6/N =&+18428658/5J_1^6+14258448J_1^5J_2+105225444/5J_1^4J_2^2+12655008J_1^3J_2^3+2874276J_1^2J_2^4\\
&+330441/5J_2^6\\
d_7/N =&-2868375573/50J_1^7-6631357068/25J_1^6J_2-12155461626/25J_1^5J_2^2-10838122554/25J_1^4J_2^3\\
&-4472334426/25J_1^3J_2^4-842315208/25J_1^2J_2^5+3957639/100J_2^7\\
d_8/N =&+114953529119/125J_1^8+612539835552/125J_1^7J_2+1339378449936/125J_1^6J_2^2\\
&+306492907024/25J_1^5J_2^3+945223599576/125J_1^4J_2^4+58819461696/25J_1^3J_2^5\\
&+8746434504/25J_1^2J_2^6+730594991/250J_2^8\\
d_9/N =&-10537864919249/700J_1^9-11295754776144/125J_1^8J_2-28650262033449/125J_1^7J_2^2\\
&-277255243051707/875J_1^6J_2^3-223354581526359/875J_1^5J_2^4-20611519986042/175J_1^4J_2^5\\
&-5096421652536/175J_1^3J_2^6-3188687017356/875J_1^2J_2^7+2133340729/1000J_2^9\\
d_{10}/N =&+124915768903309/500J_1^{10}+1458608384486006/875J_1^9J_2+480035838605933/100J_1^8J_2^2\\
&+6786525118526547/875J_1^7J_2^3+13372303182069211/1750J_1^6J_2^4+581375739195882/125J_1^5J_2^5\\
&+5932042509828219/3500J_1^4J_2^6+60310914541863/175J_1^3J_2^7\\
&+25236490352669/700J_1^2J_2^8+580872222471/3500J_2^{10}
\end{aligned}
$$

## 2.5. $S = 5/2$

Susceptibility:

$$
\begin{aligned}
c_1/N =& + 35/12 \\
c_2/N =& - 1225/12 J_1 - 1225/24 J_2 \\
c_3/N =& + 233975/72 J_1^2 + 42875/12 J_1 J_2 + 52675/72 J_2^2 \\
c_4/N =& - 42852215/432 J_1^3 - 49177625/288 J_1^2 J_2 - 11876375/144 J_1 J_2^2 - 8809465/864 J_2^3 \\
c_5/N =& + 61304748925/20736 J_1^4 + 12014869825/1728 J_1^3 J_2 + 18877459475/3456 J_1^2 J_2^2 \\
& + 695492525/432 J_1 J_2^3 + 5682565525/41472 J_2^4 \\
c_6/N =& - 10795071062293/124416 J_1^5 - 2016148561735/7776 J_1^4 J_2 - 17688372918335/62208 J_1^3 J_2^2 \\
& - 8611001631575/62208 J_1^2 J_2^3 - 591071534375/20736 J_1 J_2^4 - 454017813823/248832 J_2^5 \\
c_7/N =& + 7522815281061997/2985984 J_1^6 + 3412185811836235/373248 J_1^5 J_2 \\
& + 19271427800406985/1492992 J_1^4 J_2^2 + 1105568586850805/124416 J_1^3 J_2^3 \\
& + 4556892366820745/1492992 J_1^2 J_2^4 + 14761975773545/31104 J_1 J_2^5 \\
& + 15853905979723/663552 J_2^6 \\
c_8/N =& - 108368199171274385/1492992 J_1^7 - 277736424649599 4183/8957952 J_1^6 J_2 \\
& - 240230043615662 5823/4478976 J_1^5 J_2^2 - 2866246275877143943/5971968 J_1^4 J_2^3 \\
& - 1053142334131893691/4478976 J_1^3 J_2^4 - 549353555821340375/8957952 J_1^2 J_2^5 \\
& - 7525687305218215/995328 J_1 J_2^6 - 2786280827324267/8957952 J_2^7 \\
c_9/N =& + 297937813529490933919/143327232 J_1^8 + 305143858226085938 99/2985984 J_1^7 J_2 \\
& + 150105914835639449 0591/71663616 J_1^6 J_2^2 + 1243014974793982515517/53747712 J_1^5 J_2^3 \\
& + 1594247137860695924753/107495424 J_1^4 J_2^4 + 99422167643150752183/17915904 J_1^3 J_2^5 \\
& + 247781950159184404565/214990848 J_1^2 J_2^6 + 20891409215721017 05/17915904 J_1 J_2^7 \\
& + 3452973474116996413/859963392 J_2^8 \\
c_{10}/N =& - 15922809234031210877 41/26873856 J_1^9 - 212551008373253152284815/644972544 J_1^8 J_2 \\
& - 503886040648503953991019/644972544 J_1^7 J_2^2 - 147275596822846278581291/143327232 J_1^6 J_2^3 \\
& - 351552213386584479341429/429981696 J_1^5 J_2^4 - 519270979718558264487787/1289945088 J_1^4 J_2^5 \\
& - 155365796364173356885637/1289945088 J_1^3 J_2^6 - 88549191998419662488 65/429981696 J_1^2 J_2^7 \\
& - 3769640012333104828 45/214990848 J_1 J_2^8 - 1332361155650813248 49/2579890176 J_2^9
\end{aligned}
$$

Heat capacity:

$$
\begin{aligned}
d_1/N =& 0 \\
d_2/N =& + 1225/8J_1^2 + 1225/16J_2^2 \\
d_3/N =& - 167825/48J_1^3 - 42875/8J_1^2J_2 + 1225/32J_2^3 \\
d_4/N =& + 29449735/384J_1^4 + 557375/3J_1^3J_2 + 2100875/24J_1^2J_2^2 + 1384495/256J_2^4 \\
d_5/N =& - 5907916525/3456J_1^5 - 1502382875/288J_1^4J_2 - 510426875/96J_1^3J_2^2 - 246488375/144J_1^2J_2^3 \\
& + 18351725/6912J_2^5 \\
d_6/N =& + 6367584649055/165888J_1^6 + 501418794625/3456J_1^5J_2 + 5763760243675/27648J_1^4J_2^2 \\
& + 143868391625/1152J_1^3J_2^3 + 89332935125/3072J_1^2J_2^4 + 228542728855/331776J_2^6 \\
d_7/N =& - 292825435311577/331776J_1^7 - 82862694155815/20736J_1^6J_2 \\
& - 594582883120765/82944J_1^5J_2^2 - 521266905599965/82944J_1^4J_2^3 - 431738298942545/165888J_1^3J_2^4 \\
& - 27740750842945/55296J_1^2J_2^5 + 95904954481/221184J_2^7 \\
d_8/N =& + 165855125630193307/7962624J_1^8 + 81352449953851601/746496J_1^7J_2 \\
& + 698888405867532713/2985984J_1^6J_2^2 + 7276549571182955/27648J_1^5J_2^3 \\
& + 240338850411084061/1492992J_1^4J_2^4 + 37657927270221055/746496J_1^3J_2^5 \\
& + 1914789405843125/248832J_1^2J_2^6 + 3268207159586467/47775744J_2^8 \\
d_9/N =& - 5985138672294524471/11943936J_1^9 - 184222906294089481/62208J_1^8J_2 \\
& - 4906096516615431277/663552J_1^7J_2^2 - 60116916071401449281/5971968J_1^6J_2^3 \\
& - 7973279190092104315/995328J_1^5J_2^4 - 3670078683300269135/995328J_1^4J_2^5 \\
& - 28624433615472275/31104J_1^3J_2^6 - 58943968377184625/497664J_1^2J_2^7 \\
& + 418813879532953/7962624J_2^9 \\
d_{10}/N =& + 1556526037774175926811/127401984J_1^{10} + 1920557937785839792195/23887872J_1^9J_2 \\
& + 10906489523378708337785/47775744J_1^8J_2^2 + 45266820569196058105/124416J_1^7J_2^3 \\
& + 67669410870719638272005/191102976J_1^6J_2^4 + 2554770854887551794795/11943936J_1^5J_2^5 \\
& + 552609289173353092205/7077888J_1^4J_2^6 + 127854220349644552925/7962624J_1^3J_2^7 \\
& + 33035238778703928925/191102976J_1^2J_2^8 + 2105769000633157751/254803968J_2^{10}
\end{aligned}
$$

## 3. MULTIPLICATOR ESTIMATES CONNECTING EXCHANGE COUPLING CONSTANT WITH NEEL TEMPERATURE

TABLE S3: The multiplicator estimates $m$ of Neel temperatures $T_N = m \cdot J_2$ computed at $J_1/J_2$ ratios predicted by different methods from $\chi$ and $C$.

| | NiO, GW | | | | NiO, UHF | | | |
|---|---|---|---|---|---|---|---|---|
| $n$ | $g_n$ | $h_n$ | $f_n$ | $r_n$ | $g_n$ | $h_n$ | $f_n$ | $r_n$ |
| 2 | 2.0268 | 4.0537 | 2.0286 | 2.8688 | 1.8305 | 3.6609 | 2.0486 | 2.8971 |
| 3 | 1.9098 | 3.3078 | 1.0464 | 1.5091 | 1.5688 | 2.7173 | 0.8319 | 1.1998 |
| 4 | 1.6372 | 2.5989 | 1.5514 | 2.1940 | 0.7941 | 1.2606 | 1.6062 | 2.2715 |
| 5 | 0.8079 | 1.2080 | 1.5089 | 2.0818 | 1.7318 | 2.5896 | 1.5777 | 2.1768 |
| 6 | 1.8021 | 2.5788 | 2.1108 | 2.8454 | 1.9753 | 2.8266 | 2.1393 | 2.8838 |
| 7 | 2.0397 | 2.8211 | 1.6775 | 2.2151 | 2.0168 | 2.7894 | 1.8162 | 2.3983 |
| 8 | 2.1088 | 2.8382 | 2.0685 | 2.6825 | 1.9464 | 2.6196 | 2.1076 | 2.7333 |
| 9 | 2.1079 | 2.7741 | 1.9624 | 2.5051 | 1.7800 | 2.3426 | 2.0175 | 2.5753 |
| 10 | 2.0538 | 2.6526 | 2.2085 | 2.7803 | 1.6198 | 2.0920 | 2.2326 | 2.8107 |
| | NiO, DDCI2 | | | | NiO, DDCI3 | | | |
| $n$ | $g_n$ | $h_n$ | $f_n$ | $r_n$ | $g_n$ | $h_n$ | $f_n$ | $r_n$ |
| 2 | 2.1587 | 4.3175 | 2.0181 | 2.8540 | 2.0777 | 4.1554 | 2.0242 | 2.8627 |
| 3 | 2.1216 | 3.6748 | 1.1326 | 1.6335 | 1.9928 | 3.4516 | 1.0834 | 1.5625 |
| 4 | 1.9617 | 3.1140 | 1.5125 | 2.1390 | 1.7709 | 2.8111 | 1.5364 | 2.1728 |
| 5 | 1.6924 | 2.5308 | 1.4424 | 1.9901 | 1.2708 | 1.9003 | 1.4851 | 2.0491 |
| 6 | 0.9837 | 1.4077 | 2.0872 | 2.8136 | 1.6754 | 2.3974 | 2.1020 | 2.8335 |
| 7 | 1.8866 | 2.6093 | 1.5048 | 1.9871 | 2.0066 | 2.7752 | 1.6238 | 2.1442 |
| 8 | 2.0904 | 2.8135 | 2.0335 | 2.6371 | 2.1166 | 2.8487 | 2.0559 | 2.6662 |
| 9 | 2.1718 | 2.8583 | 1.9055 | 2.4324 | 2.1450 | 2.8230 | 1.9432 | 2.4805 |
| 10 | 2.1905 | 2.8291 | 2.1878 | 2.7543 | 2.1210 | 2.7393 | 2.2012 | 2.7711 |
| | NiO, CASSCF | | | | NiO, CASPT2 | | | |
| $n$ | $g_n$ | $h_n$ | $f_n$ | $r_n$ | $g_n$ | $h_n$ | $f_n$ | $r_n$ |
| 2 | 2.1333 | 4.2667 | 2.0199 | 2.8566 | 2.2834 | 4.5669 | 2.0103 | 2.8430 |
| 3 | 2.0817 | 3.6056 | 1.1183 | 1.6129 | 2.3133 | 4.0068 | 1.1897 | 1.7158 |
| 4 | 1.9042 | 3.0228 | 1.5200 | 2.1495 | 2.2218 | 3.5268 | 1.4769 | 2.0887 |
| 5 | 1.5871 | 2.3733 | 1.4564 | 2.0095 | 2.0825 | 3.1141 | 1.3655 | 1.8840 |
| 6 | 1.3903 | 1.9895 | 2.0919 | 2.8199 | 1.9239 | 2.7530 | 2.0633 | 2.7814 |
| 7 | 1.9368 | 2.6788 | 1.5484 | 2.0446 | 1.5616 | 2.1598 | 1.0374 | 1.3699 |
| 8 | 2.1049 | 2.8330 | 2.0409 | 2.6467 | 1.8278 | 2.4600 | 1.9922 | 2.5836 |
| 9 | 2.1681 | 2.8534 | 1.9184 | 2.4489 | 2.0925 | 2.7538 | 1.8214 | 2.3250 |
| 10 | 2.1733 | 2.8069 | 2.1923 | 2.7600 | 2.2001 | 2.8415 | 2.1622 | 2.7221 |

TABLE S4: The multiplicator estimates $m$ of Neel temperatures $T_N = m \cdot J_2$ computed at $J_1/J_2$ ratios predicted by different methods from $\chi$ and $C$.

| | CoO, GW | | | | CoO, UHF | | | |
|---|---|---|---|---|---|---|---|---|
| $n$ | $g_n$ | $h_n$ | $f_n$ | $r_n$ | $g_n$ | $h_n$ | $f_n$ | $r_n$ |
| 2 | 7.5217 | 15.043 | 3.7865 | 5.3549 | 4.2334 | 8.4669 | 4.0221 | 5.6881 |
| 3 | 5.5608 | 9.6317 | 1.4686 | 2.1181 | 1.3564 | 2.3493 | 2.6769 | 3.8608 |
| 4 | 4.7617 | 7.5587 | 3.4929 | 4.9397 | 3.9932 | 6.3388 | 3.8279 | 5.4135 |
| 5 | 4.0611 | 6.0728 | 2.5201 | 3.4770 | 4.1401 | 6.1908 | 3.3212 | 4.5824 |
| 6 | 3.0597 | 4.3783 | 4.0453 | 5.4531 | 3.4179 | 4.8910 | 4.2603 | 5.7430 |
| 7 | 3.8130 | 5.2738 | 3.3125 | 4.3740 | 3.3036 | 4.5691 | 4.0635 | 5.3657 |
| 8 | 4.3351 | 5.8347 | 4.1412 | 5.3704 | 3.7973 | 5.1108 | 4.4596 | 5.7834 |
| 9 | 4.5294 | 5.9610 | 3.7876 | 4.8350 | 3.5760 | 4.7063 | 4.3642 | 5.5710 |
| 10 | 4.5802 | 5.9155 | 4.3098 | 5.4258 | 4.1954 | 5.4186 | 4.6055 | 5.7979 |

TABLE S5: The multiplicator estimates $m$ of Neel temperatures $T_N = m \cdot J_2$ computed at $J_1/J_2$ ratios predicted by different methods from $\chi$ and $C$. 5x5x5 k-point grid is used.

| | FeO, GW | | | | FeO, UHF | | | |
|---|---|---|---|---|---|---|---|---|
| $n$ | $g_n$ | $h_n$ | $f_n$ | $r_n$ | $g_n$ | $h_n$ | $f_n$ | $r_n$ |
| 2 | 10.440 | 20.880 | 6.4611 | 9.1374 | 7.0603 | 14.121 | 8.1332 | 11.5020 |
| 3 | 2.8504 | 4.9371 | 4.5589 | 6.5750 | 8.6197 | 14.930 | 7.3875 | 10.6546 |
| 4 | 7.3568 | 11.678 | 6.4663 | 9.1447 | 6.9818 | 11.083 | 5.1083 | 7.22417 |
| 5 | 7.3985 | 11.063 | 5.6559 | 7.8036 | 7.3392 | 10.975 | 5.6600 | 7.80923 |
| 6 | 6.1235 | 8.7626 | 7.0272 | 9.4727 | 6.3398 | 9.0721 | 7.5380 | 10.1613 |
| 7 | 5.2772 | 7.2988 | 6.7357 | 8.8942 | 7.3964 | 10.230 | 8.4946 | 11.2169 |
| 8 | 6.3397 | 8.5326 | 7.3677 | 9.5547 | 4.4781 | 6.0271 | 8.5641 | 11.1063 |
| 9 | 6.0047 | 7.9026 | 7.2396 | 9.2415 | 7.1632 | 9.4274 | 8.2409 | 10.5197 |
| 10 | 5.1386 | 6.6368 | 7.6041 | 9.5730 | 6.3604 | 8.2148 | 8.2826 | 10.4272 |

TABLE S6: The multiplicator estimates $m$ of Neel temperatures $T_N = m \cdot J_2$ computed at $J_1/J_2$ ratios predicted by different methods from $\chi$. The found values are consistent with Ref.[4].

| | MnO, GW | | | MnO, UHF | | |
|---|---|---|---|---|---|---|
| $n$ | $q_n$ | $g_n$ | $h_n$ | $q_n$ | $g_n$ | $h_n$ |
| 2 | 56.9694 | 166.161 | 332.321 | 61.2612 | 178.679 | 357.357 |
| 3 | 53.5225 | 94.3045 | 163.340 | 57.5283 | 101.386 | 175.605 |
| 4 | 52.1636 | 77.4125 | 122.885 | 56.1043 | 83.2370 | 132.131 |
| 5 | 50.9828 | 69.7371 | 104.281 | 54.6297 | 74.9195 | 112.031 |
| 6 | 50.5392 | 65.3878 | 93.5679 | 54.2272 | 70.2294 | 100.496 |
| 7 | 50.1226 | 62.5537 | 86.5172 | 53.7709 | 67.1723 | 92.9052 |
| 8 | 49.8117 | 60.5510 | 81.4956 | 53.4311 | 65.0116 | 87.4991 |
| 9 | 49.5707 | 59.0554 | 77.7212 | 53.1682 | 63.3977 | 83.4361 |
| 10 | 49.3785 | 57.8927 | 74.7713 | 52.9586 | 62.1429 | 80.2607 |

TABLE S7: The multiplicator estimates $m$ of Neel temperatures $T_N = m \cdot J_2$ computed at $J_1/J_2$ ratios predicted by different methods from $C$.

| | MnO, GW | | | MnO, UHF | | |
|---|---|---|---|---|---|---|
| $n$ | $q_n$ | $f_n$ | $r_n$ | $q_n$ | $f_n$ | $r_n$ |
| 2 | | 16.4709 | 23.2934 | | 17.7748 | 25.1373 |
| 3 | 43.4637 | 22.7608 | 32.8267 | 48.0280 | 24.7572 | 35.7060 |
| 4 | 43.0145 | 26.6867 | 37.7406 | 45.6591 | 28.8508 | 40.8012 |
| 5 | 42.1002 | 29.2343 | 40.3354 | 44.7991 | 31.5050 | 43.4684 |
| 6 | 42.0289 | 31.0576 | 41.8659 | 44.7743 | 33.4058 | 45.0312 |
| 7 | 42.1998 | 32.4480 | 42.8466 | 45.0577 | 34.8647 | 46.0377 |
| 8 | 42.5406 | 33.5653 | 43.5288 | 45.4750 | 36.0420 | 46.7407 |
| 9 | 42.9002 | 34.4930 | 44.0310 | 45.8929 | 37.0227 | 47.2602 |
| 10 | 43.2380 | 35.2813 | 44.4166 | 46.2751 | 37.8579 | 47.6602 |

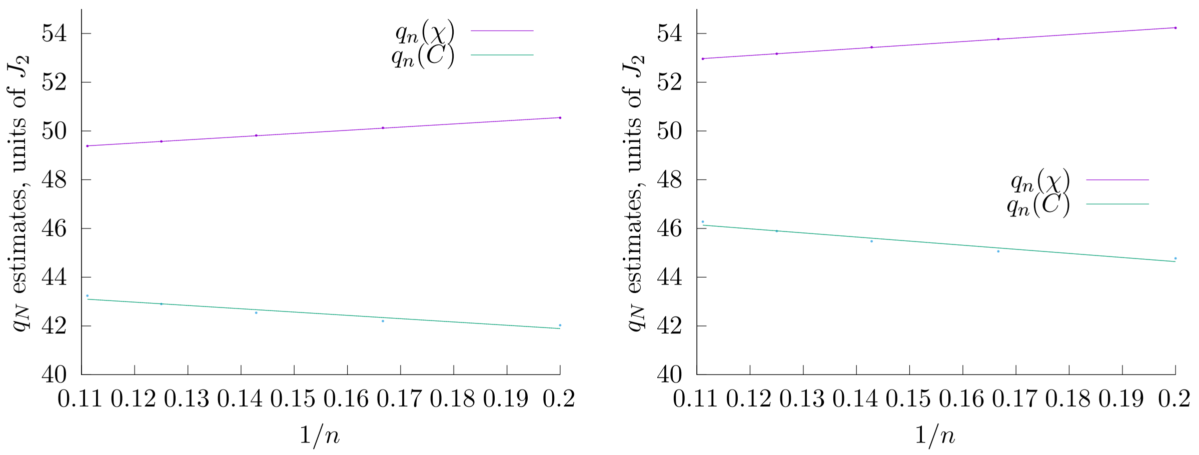


FIG. S1: Left: GW; Right: UHF. MnO dependence of $q_n$ vs $1/n$ and their linear fit, known as Domb–Sykes plot. The resulting linear fits are $q_n(\chi) = (13.0478 \pm 0.1534)\frac{1}{n} + (47.9388 \pm 0.02338)$, $q_n(C) = (-13.5415 \pm 2.25)\frac{1}{n} + (44.6009 \pm 0.3429)$ for GW and $q_n(\chi) = (14.2607 \pm 0.1596)\frac{1}{n} + (51.3845 \pm 0.02433)$, $q_n(C) = (-16.82 \pm 2.23)\frac{1}{n} + (48.0033 \pm 0.3399)$ for UHF. The indicated errors are asymptotic standard errors.

[1] G. S. Rushbrooke and P. J. Wood, On the high-temperature susceptibility for the Heisenberg model of a ferromagnet, Proc. Phys. Soc. A **68**, 1161 (1955).

[2] C. Domb and M. F. Sykes, On the susceptibility of a ferromagnetic above the Curie point, Proc. R. Soc. Lond. A **240**, 214 (1957).

[3] M. Troyer, F. Alet, and S. Wessel, Histogram methods for quantum systems: from reweighting to Wang-Landau sampling, Braz. J. Phys. **34**, 377 (2004).

[4] D. W. Wood and N. W. Dalton, Ferromagnetic Curie temperatures of the Heisenberg model with next-nearest-neighbor interactions, Phys. Rev. **159**, 384 (1967).
